# Supplementary material for: Zhyper: Factorized Hypernetworks for Conditioned LLM Fine-Tuning
Source: arXiv:2510.19733 source file (2025-10-23)
Supplement: Supplementary file 1 [file A.tex]

\section{Additional Experiments}
You may include other additional sections here.

\section{Broader Impact / Limitations}
